# Supplementary material for: GateKeeper-GPU: Fast and Accurate Pre-Alignment Filtering in Short Read Mapping
Source: arXiv:2103.14978 source file (2024-02-22)
Supplement: Supplementary file 2 [file appendices.tex]

% if have a single appendix:
%\appendix[Proof of the Zonklar Equations]
% or
%\appendix  % for no appendix heading
% do not use \section anymore after \appendix, only \section*
% is possibly needed

% use appendices with more than one appendix
% then use \section to start each appendix
% you must declare a \section before using any
% \subsection or using \label (\appendices by itself
% starts a section numbered zero.)
%

\appendices
Appendix one text goes here.

% you can choose not to have a title for an appendix
% if you want by leaving the argument blank
\section{}
